# Supplementary material for: Non-collinear spin-orbit magnetic fields in a carbon nanotube double quantum dot
Source: arXiv:1606.01065 source file (2016-06-03)
Supplement: Supplementary file 1 [file supplement.pdf]

# Non-collinear spin-orbit magnetic fields in a carbon nanotube double quantum dot

## Supplemental Information

M. C. Hels,[1] B. Braunecker,[2] K. Grove-Rasmussen,[1] and J. Nygård[1]

[1] Center for Quantum Devices and Nano-Science Center, Niels Bohr Institute, University of Copenhagen, Universitetsparken 5, 2100 Copenhagen Ø, Denmark

[2] SUPA, School of Physics and Astronomy, University of St. Andrews, North Haugh, St. Andrews KY16 9SS, United Kingdom

(Dated: May 17, 2016)

While we could clearly demonstrate that our device has spin polarized quantum dot levels, they are not fully polarized mainly due to scattering between the valleys $K$ and $K'$. This degradation of the spin polarization has substantial influence on spin entanglement detection schemes and can lead to erroneous conclusions. In this supplement we provide an estimate on the acceptable magnitude of the inter-valley scattering. Remarkably, our current device is close to fulfilling the necessary requirements for entanglement detection.

For transport measurements in the Cooper pair splitter, we shall focus on the entanglement detection scheme put forward in Ref. [S1]. It relies on the violation of the CSHS Bell inequality

$$Q = |\langle S_K S'_K \rangle + \langle S_K S'_{K'} \rangle + \langle S_{K'} S'_K \rangle - \langle S_{K'} S'_{K'} \rangle| \leq 2, \quad \text{(S1)}$$

which includes four nonlocal spin correlators obtained, as described below, by transport measurements through the different quantum dot levels. Equation (S1) was originally designed to disprove, for instance, hidden variable theories. However, if we accept quantum mechanics, a violation of Eq. (S1), i.e. a measurement of $Q > 2$, provides a sufficient demonstration of the existence of entanglement in the measured quantum states, which are in the present setup the split spin-entangled Cooper pairs.

This detection of entanglement is robust against most scattering processes and imperfections in either quantum dot, but can be falsified by inter-valley scattering $\Delta_{KK'}$ [S1]. While the latter is unimportant for semiconducting nanotubes [S1], it plays a limiting role for the small bandgap nanotubes used in the experiments. In the following we will use $Q'$ to denote the result for Eq. (S1) in the presence of $\Delta_{KK'}$ and use $Q$ for the ideal, unperturbed value. In Fig. S1 we show $Q'$ as a function of magnetic field rotation angle $\varphi$ for the parameters of shells h and N provided in the main text, comparing the calculated values $Q'$ for the experimentally determined $\Delta_{KK'}$ (dashed lines) with the optimal case of $\Delta_{KK'} = 0$ in both dots (solid lines), assuming the injection of spin singlet electron pairs in the Cooper pair splitter. Figure S1 shows that the valley mixing is dominating $Q'$ and that the violation of Eq. (S1) does not allow any conclusion on the entanglement of the injected electron pairs. In particular, the fact that $Q'$ exceeds the maximally possible value $Q = \sqrt{8} \approx 2.83$ for spin correlators demonstrates that the spin reconstruction completely fails. The relevant question is therefore about the acceptable maximum $\Delta_{KK'}$ such that Eq. (S1) remains trustworthy for entanglement detection.

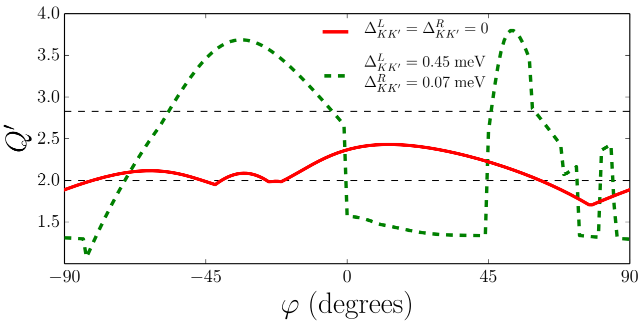


FIG. S1: Values of $Q'$, evaluated by Eq. (S1) in the presence of $\Delta_{KK'}$, as a function of the magnetic field rotation angle $\varphi$, based on the effective model with the experimentally determined parameters for shells h (left quantum dot $L$) and N (right quantum dot $R$), computed for the splitting of spin-singlet entangled Cooper pairs at $B = 0.7$ T and the angle $\Delta\varphi_{\text{SO}} = 21^\circ$ between the quantum dot axes. The solid red line shows the ideal case $Q' = Q$ with $\Delta^L_{KK'} = \Delta^R_{KK'} = 0$, and shows over a wide range $2 < Q < \sqrt{8} \approx 2.83$ (between the dashed horizontal lines), demonstrating the potential of this Cooper pair splitter for entanglement detection. The dashed green line represents the same calculation of $Q'$ in the presence of $\Delta^L_{KK'} = 0.45$ meV for shell h and $\Delta^R_{KK'} = 0.07$ meV for shell N, which are strong enough scattering amplitudes to destroy the resemblance with the red curve and lead even to $Q' > \sqrt{8}$ which would be impossible for spin correlators.

In the following we answer this question by first identifying the situations in which $\Delta_{KK'}$ scattering can become decisive, which requires an investigation of the microscopic model of carbon nanotubes. This will provide us estimates on the acceptable magnitudes of $\Delta_{KK'}$. These estimates are then corroborated by some quantitative numerical examples. Our main conclusion is that even small bandgap nanotubes remain useful for entanglement detection under considerable amounts of inter-valley scattering, if a careful selection of the angular range is made where the individual levels remain energetically far apart with respect to the $\Delta_{KK'}$.

For the experiment presented this means that the right side (shell N) has sufficiently low valley mixing, while the left side (shell h) should be in the same regime, i.e. in the sub 100 $\mu$eV range. This is an experimentally challenging but feasible requirement. Furthermore, even for larger $K - K'$ coupling, the strong variations of $Q$ seen in Fig. S1 may be tested and would provide insight into the applicability of the model and the assumption

related to tunneling.

### Effect of valley mixing on spin projections

If we neglect spin-orbit interaction (SOI), curvature and inter-valley scattering, the 4 levels of a quantum dot orbital, for 2 spin projections $s = +,- =\uparrow,\downarrow$ and 2 valley indices $\tau = +,- = K, K'$, have degenerate energies $E_{\tau,s}$. If we choose the spin $S_z$ direction along the nanotube axis, SOI and curvature cause a partial lifting of the degeneracy, such that $E_{\tau,s} \neq E_{\tau,-s}$, but $E_{\tau,s} = E_{-\tau,-s}$ is maintained due to the time-reversal symmetry of the SOI. Nonetheless, the splitting can be interpreted as arising from a valley dependent Zeeman field $\tau B_{\rm SO}\hat{\mathbf{z}}$, where $\hat{\mathbf{z}}$ is the unit vector along the nanotube axis. The further application of an external magnetic field $\mathbf{B}$ then creates an effective, valley dependent Zeeman field $\mathbf{B}_\tau^{\rm eff} = \mathbf{B} + \tau B_{\rm SO}\hat{\mathbf{z}}$. The orbital effect of the magnetic field causes a further valley dependent shift of the energy levels, expressible by an orbital $g$-factor $\tau g_{\rm orb}$ (with a positive or negative $g_{\rm orb}$ depending on whether the quantum dot is electron like or hole like) multiplying the $z$ component of the magnetic field. Consequently, the effective Hamiltonian describing the quantum dot in a magnetic field takes the form

$$H_0 = E_0 + \frac{g_s}{2}\mu_B \mathbf{S}\cdot(\mathbf{B} + \tau_z B_{\rm SO}\hat{\mathbf{z}}) - \tau_z g_{\rm orb}\hat{\mathbf{z}}\cdot\mathbf{B}, \quad \text{(S2)}$$

for $E_0$ an energy offset, $\mathbf{S} = (S_x, S_y, S_z)$ the vector of spin-Pauli matrices, and we will use $\tau_{x,y,z}$ for the valley Pauli matrices. Both Zeeman and orbital effects together cause a full lifting of the degeneracy, and hence allow the detection of each state individually. Due to the Zeeman term, each eigenstate is fully spin polarized, providing a projection onto $\pm S_\tau$ where $S_\tau = \hat{\mathbf{a}}_\tau \cdot \mathbf{S}$ for $\hat{\mathbf{a}}_\tau = \mathbf{B}_\tau^{\rm eff}/|\mathbf{B}_\tau^{\rm eff}|$ the unit vector parallel to $\mathbf{B}_\tau^{\rm eff}$. As shown in Ref. [S1], the reconstruction of spin correlators through conductance measurements over these spin projective states can be used to probe the spin entanglement of Cooper pairs in a Cooper pair splitter setup through a Bell inequality as Eq. (S1).

The requirement for a useful test of the Bell inequality are measurements along non-collinear spin projection axes $\hat{\mathbf{a}}_K$ and $\hat{\mathbf{a}}_{K'}$. A valley mixing scattering process with amplitude $\Delta_{KK'}$ leads to a hybridization between the different spin projected eigenstates. Spin is then no longer a good quantum number, and the interpretation of the Bell inequality becomes for large $\Delta_{KK'}$ meaningless. For a quantitative estimate, we need to investigate the effect of $\Delta_{KK'}$.

For this purpose, we must consider the Hamiltonian before attaining the effective model of Eq. (S2). Following the notations of Refs. [S2, S3], the Hamiltonian of a long carbon nanotube is given by

$$H_{\rm CNT} = \hbar v_F\big(k_G\sigma_1 + k'\tau_z\sigma_2\big) + \big(\alpha\sigma_1 + \beta\tau_z\big)S_z, \quad \text{(S3)}$$

where $v_F$ is the Fermi velocity, $\sigma_{1,2}$ the Pauli matrices referring to the $A, B$ sublattice indices of the hexagonal carbon lattice, and $\alpha, \beta$ are the SOI coupling constants (denoted by $\Delta^1_{\rm SO}, \Delta^0_{\rm SO}$ in Ref. [S4]), depending both on chirality and radius. The quantity $k' = k + \Delta k^z_{cv}$ denotes the sum of the longitudinal momentum $k$ and a small curvature induced shift $\Delta k^z_{cv}$. Finally, $k_G = k^0_G + \Delta k^t_{cv}$ provides the transverse quantized momentum, giving rise to the gap $E_G = 2\hbar v_F k_G$ between the subbands, with $\Delta k^t_{cv}$ a curvature induced offset and $k^0_G = (n - \tau m/3)/R$ for $n$ the subband index, $R$ the nanotube radius, and $m = (N_1 - N_2)$ mod 3, for the chirality indices $(N_1, N_2)$. The confinement potential of a quantum dot causes a further quantization of $k'$ and leads to the quantum dot levels that can be captured by the effective Hamiltonian $H_0$, with level depending $B_{\rm SO}$, $E_0$, and $g_{\rm orb}$.

For the lowest subband $n = 0$, it is important to notice that both $k^0_G$ and $\Delta k^t_{cv}$ [S2, S3] are proportional to $\tau$ and hence have opposite signs in opposite valleys (yet the final eigenvalues depend on the squares of these amplitudes and lead to similar energies in each valley). A valley mixing scattering potential of the form $H_{KK'} = \tau_x\Delta_{KK'}/2$ leads therefore to a mixing of components in the Hamiltonian that are characterized by the energy amplitudes $+E_G$ and $-E_G$. In the limit $|\Delta_{KK'}| \ll |E_G|$, the hybridization between the valleys can be expanded as a function of $\Delta_{KK'}/E_G$. With typical values $\Delta_{KK'} \sim 0.1$ meV, it is clear that for semiconducting nanotubes with $E_G \sim 100$ meV the effect of the hybridization is negligible [S1], and Hamiltonian (S2) as well as its consequences, for instance, on probing the Bell inequality remain unchanged.

However, for small gap nanotubes with $k^0_G = 0$, the dominating role of $E_G$ is replaced by a competition between $\Delta_{KK'}$ with the remaining curvature induced bandgap, the SOI coupling strength, the quantum dot confinement energy, and the orbital and Zeeman energies by the magnetic field, which all together lead to the effective magnetic splittings $|g_S\mu_B\mathbf{B}^{\rm eff}_\tau|$ and $|2g_{\rm orb}\mu_B\hat{\mathbf{z}}\cdot\mathbf{B}|$. As long as $\Delta_{KK'}$ remains smaller than these scales, the loss of spin polarization by the valley mixing remains a small effect. It should be noticed that the curvature induced small gap $\hbar v_F\Delta k^t_{cv}$ depends on the nanotube diameter $D$ as $\Delta k^t_{cv} \propto 1/D^2$, allowing us to achieve some tuneability of $\mathbf{B}^{\rm eff}_\tau$ by choosing nanotubes with smaller or larger diameter.

The preceding observations can be quantified by adding the first order correction in $H_{KK'}$ to the wave functions,

$$|\psi_{\tau,s}\rangle = |\phi_{\tau,s}\rangle + \sum_{s'} \frac{\langle\phi_{-\tau,s'}|\Delta_{KK'}\tau_x|\phi_{\tau,s}\rangle}{E_{\tau,s} - E_{-\tau,s'}}|\phi_{-\tau,s'}\rangle, \quad \text{(S4)}$$

where $|\phi_{\tau,s}\rangle$ and $E_{\tau,s}$ denote the eigenvectors and eigenvalues of $H_0$. If $\chi$ is the angle between $\hat{\mathbf{a}}_K$ and $\hat{\mathbf{a}}_{K'}$, we have $\langle\phi_{-\tau,s'}|\Delta_{KK'}\tau_x|\phi_{\tau,s}\rangle \propto \cos(\chi/2)$ for $s = s'$ and $\propto \sin(\chi/2)$ for $s \neq s'$. For general angles $\cos(\chi/2), \sin(\chi/2) \sim 1$, showing that the amplitude of the valley mixing part of the wave function is indeed set by $\delta_\tau = \Delta_{KK'}/\min_{s,s'}\{|E_{\tau,s} - E_{-\tau,s'}|\}$.

The ideal determination of spin expectation values is based on the projectors $P_{\tau,s} = |\phi_{\tau,s}\rangle\langle\phi_{\tau,s}|$, such that

$P_{\tau,\uparrow}-P_{\tau,\downarrow}=S_\tau=\hat{\mathbf{a}}_\tau\cdot\mathbf{S}$. For a realistic measurement, the projection is obtained from restricting transport through a selected quantum dot level, for instance, by integrating the conductance over the resonance of the level. This results in a measured quantity $G_{\tau,s}\propto\langle\phi_{\tau,s}|\hat{\rho}\hat{I}|\phi_{\tau,s}\rangle$, where $\hat{\rho}$ is the density matrix of injected particles or Cooper pairs, and $\hat{I}$ the current operator. The spin reconstruction is then based on [S1]

$$\frac{G_{\tau,\uparrow}-G_{\tau,\downarrow}}{G_{\tau,\uparrow}+G_{\tau,\downarrow}}=\langle S_\tau\rangle+\langle X_\tau\rangle, \tag{S5}$$

where the division by the sum of the $G_{\tau,s}$ provides the normalization, $\langle S_\tau\rangle$ is the ideal spin measurement, and $\langle X_\tau\rangle\sim\delta_\tau$ is the error from valley mixing.

Spin correlation measurements in a Cooper pair splitting operation are obtained in a similar way. We use the notations above for the left quantum dot and use a tilde for the quantities of the right quantum dot. If $G_{\tau,s;\tilde{\tau},\tilde{s}}$ contains the nonlocal Cooper pair splitting amplitude, projected on states $|\psi_{\tau,s}\rangle$ on the left and $|\tilde{\psi}_{\tilde{\tau},\tilde{s}}\rangle$ on the right quantum dot [S1], we have

$$\frac{\sum_{s,\tilde{s}}s\tilde{s}G_{\tau,s;\tilde{\tau},\tilde{s}}}{\sum_{s,\tilde{s}}G_{\tau,s;\tilde{\tau},\tilde{s}}}=\langle S_\tau\tilde{S}_{\tilde{\tau}}\rangle+\langle X_{\tau;\tilde{\tau}}\rangle, \tag{S6}$$

with the error $\langle X_{\tau;\tilde{\tau}}\rangle\sim\max_{\tau,\tilde{\tau}}\{\delta_\tau,\tilde{\delta}_{\tilde{\tau}}\}$. The value $Q$ in Eq. (S1) then becomes $Q'=Q+\delta Q$ with the ideal result $Q$ and the error

$$\delta Q=C\max_{\tau,\tilde{\tau}}\{\delta_\tau,\tilde{\delta}_{\tilde{\tau}}\}, \tag{S7}$$

where $C$, with $|C|\gtrsim 1$, accounts for all further details and the sums and differences in $Q$.

With such a $\delta Q$ the threshold for entanglement detection increases. Indeed, for an ideal measurement of $Q$, spin entanglement of injected electron pairs is detected if $Q\leq 2$ is violated. With a measured $Q'=Q+\delta Q$, this inequality becomes

$$Q'\leq 2+|\delta Q|, \tag{S8}$$

where we need to choose absolute values for $\delta Q$ to rule out misinterpretations of $Q'>2-|\delta Q|$ but still $Q'<2$ as proofs of entanglement. The latter equation gives an estimate on the necessary violation of the Bell inequality (S1) for a valid detection of entanglement.

It should be stressed that for large $\Delta_{KK'}$ the perturbative result (S7) is no longer limiting, and $\delta Q$ can become large and, in particular, can lead to a $Q'$ exceeding the possible maximum $Q=\sqrt{8}$ for spin correlators. The latter case is a strong indicator of a loss of spin polarization due to $\Delta_{KK'}$.

### Quantitative numerical test

For a quantitative check of the estimate in Eq. (S8) we investigate the influence of $\Delta_{KK'}$ on two models of the type as discussed above. As the first example, we consider a nanotube with chirality (24,12) in a magnetic field of $B=1$ T, in a bent Cooper pair splitter setup as considered in Ref. [S1]. The calculation of the quantum dot levels follows then from Eq. (S3) in the presence of confining gates defining dots with a length of 450 nm, following Refs. [S1, S5–S7].

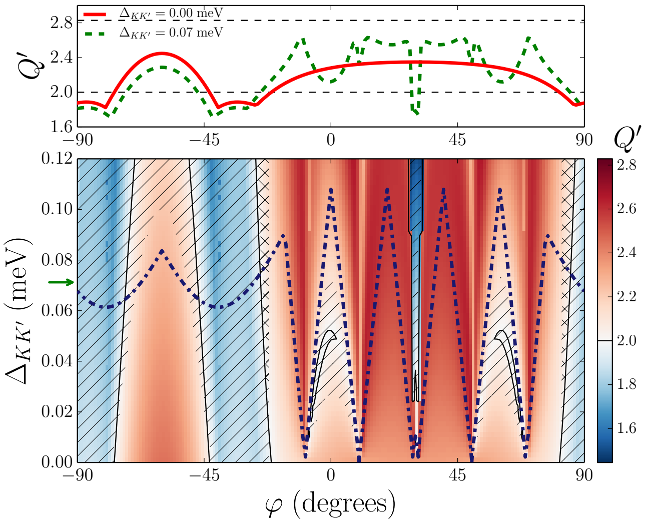


FIG. S2: The bottom graph shows a density plot for $Q'$ as a function of $\Delta_{KK'}$ (same for both quantum dots) and magnetic field angle $\varphi$ for a (24,12) nanotube in a 1 T magnetic field, with quantum dot lengths of 450 nm. Assumed is a bending angle $\Delta\varphi_{\mathrm{SO}}=30^\circ$ between both quantum dot axes and a large bending radius, as in the experimental setup, such that the local spin axes defining $\mathbf{S}$ are adiabatically transformed when transporting a spin from the left to the right end of the nanotube, such that the spin correlators in Eq. (S1) must be evaluated in the *local* coordinate systems of both quantum dots. The contour lines mark the boundary $Q'=2$. In the unhatched areas $Q'>2+|\delta Q|$ such that entanglement detection based on $Q'$ would be consistent with the ideal $Q$. In the diagonally hatched areas $Q'<2+|\delta Q|$ and no conclusion can be made. In the cross-hatched areas the ideal $Q\leq 2$ excludes entanglement detection, but $Q'>2$ due to the valley mixing, which would lead to a false entanglement detection. The dash-dotted blue line marks $\min\{\delta_\tau,\tilde{\delta}_{\tilde{\tau}}\}=1$, and the spin correlation reconstruction via Eq. (S6) is valid only far below this dash-dotted line. In the top plot we display the ideal curve with $\Delta_{KK'}=0$ (solid red line) and the curve with $\Delta_{KK'}=0.07$ meV for both quantum dots (dashed green line), corresponding to horizontal cuts through the bottom plot at the minimum and at the position of the green arrow on the vertical axis. The range of $2<Q<\sqrt{8}$ is framed by the dashed horizontal lines.

Figure S2 shows the values of $Q'$ as a function of $\varphi$ and $\Delta_{KK'}$, up to the maximum of $\Delta_{KK'}=0.12$ meV. The thick dash-dotted line marks where $\max_{\tau,\tau'}\{\delta_\tau,\delta'_{\tau'}\}=1$, and we can expect that the entanglement detection remains valid sufficiently below this line. In the diagonally dashed regions $Q<2+|\delta Q|$ and entanglement detection is impossible, whereas in the undashed regions $Q>2+|\delta Q|$ provides a safe entanglement detection. The cross-hatching, however, marks regions, in which $Q'>2$ but $Q<2$, meaning that $|\delta Q|$ is large enough to provide an apparent but de facto inconclusive violation of the Bell inequality. The black contour lines mark the threshold

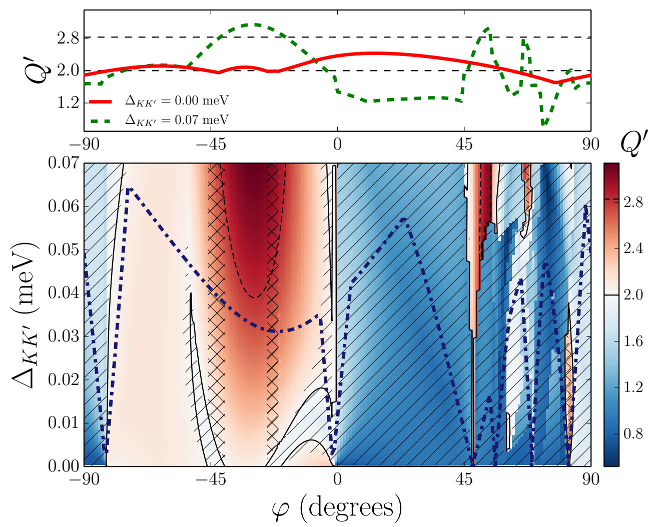


FIG. S3: Same plots as for Fig. S2 based on the effective model, Eq. (S2), for both quantum dots with the experimental parameters for shells h (hole type, $\Delta_{SO} = g_s\mu_B B_{SO}/2 = 0.05$ meV, $g_{orb} = 5.2$, $g_s = 2$) and N (electron type, $\Delta_{SO} = 0.15$ meV, $g_{orb} = 2.6$, $g_s = 2$), subject to $B = 0.7$ T and the bending angle $\Delta\varphi_{SO} = 21°$. The dashed contour lines show where $Q'$ exceeds the nominal maximum $Q = 2\sqrt{2}$, giving a definite identification of the regions where the spin correlation reconstruction is entirely invalidated due to $\Delta_{KK'}$.

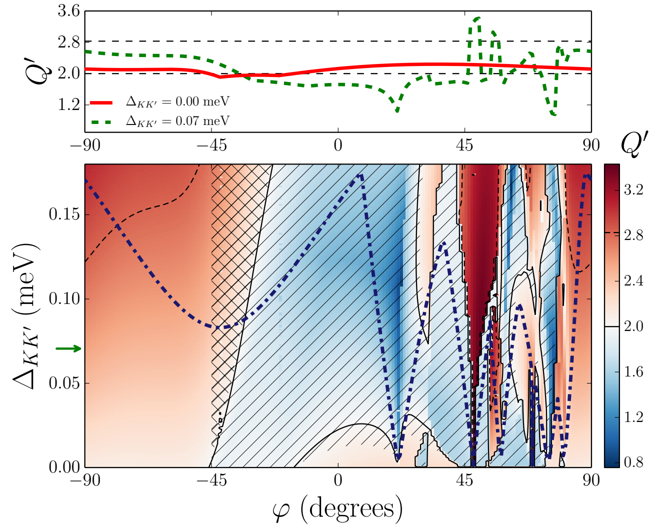


FIG. S4: Repetition of the results of Fig. S3 for an increased magnetic field of $B = 2$ T and an enhanced range of $\Delta_{KK'}$. The top plot shows still the curves at $\Delta_{KK'} = 0$ and $\Delta_{KK'} = 0.07$ meV (corresponding to a horizontal cut at the green arrow on the $\Delta_{KK'}$ axis in the bottom plot).

value $Q' = 2$. This figure indicates that while for specific level configurations even weak valley mixing amplitudes of $\Delta_{KK'} \gtrsim 0.01$ meV have a sufficient influence to destroy the spin projections, the principal detectability of entanglement extends over a remarkably wide range of $\Delta_{KK'}$ values. This is illustrated in particular by the top part of Fig. S2, which shows the angular dependence of $Q'$ for the ideal case with $\Delta_{KK'} = 0$ (solid red line) and with $\Delta_{KK'} = 0.07$ meV (dashed green line). Although $Q'$ with large $\Delta_{KK'}$ shows strong jumps whenever two dot levels are coming close to each other, the overall trend and shape of the curve as a function of $\varphi$ follows the ideal case $Q$.

As a second example we consider the effective model of Eq. (S2) for a quantum dot, as used in Ref. [S4], parametrizing the spin-orbit interaction strength by the energy $\Delta_{SO} = g_s\mu_B B_{SO}/2$ and $g_{orb} \to \pm g_{orb}$ depending if the quantum dot levels are electron or hole like. Figure S3 shows the results as in Fig. S2 within this model for the experimentally determined parameters for shells h and N of the two quantum dots, yet with varying (and identical) $\Delta_{KK'}$ for both dots. In contrast to the previous example, both quantum dots are substantially different. The influence of $\Delta_{KK'}$ is much more pronounced, leading to much wider regions of inconclusive or wrong entanglement detection, also well illustrated by the inset where the curve at $\Delta_{KK'} = 0.07$ meV (dashed line) has now only little in common with the result at $\Delta_{KK'} = 0$ (solid line).

Yet improvement can be made even for this system, for instance, by enhancing the stability of the spin polarizations by increasing the magnetic field (assuming that the critical field for the superconductor could be increased accordingly). Figure S4 shows the same situation as Fig. S3 for the larger field $B = 2$ T. While still far from ideal, the improvement of the situation for entanglement detection is quite notable.

These results show that with the flexibility of the free choice of $\varphi$ there are ranges of the direction of the magnetic field, in which $Q'$ follows quite closely the ideal values of $Q$ even for values of $\Delta_{KK'}$ that can become even as large as the 0.07 meV of shell N. From the data these angular ranges are characterized by a smooth behavior of $Q'$ without the discontinuous jumps arising from approaching and crossing energy levels, for which the strict requirement $\Delta_{KK'} \ll \min_{\tau,s,s'}\{|E_{\tau,s} - E_{-\tau,s'}|\}$ can be weakened to $\Delta_{KK'}$ approaching this upper limit.


[S1] B. Braunecker, P. Burset, and A. Levy Yeyati, Phys. Rev. Lett. **111**, 136806 (2013).
[S2] J. Klinovaja, M. J. Schmidt, B. Braunecker, and D. Loss, Phys. Rev. Lett. **106**, 156809 (2011).
[S3] J. Klinovaja, M. J. Schmidt, B. Braunecker, and D. Loss, Phys. Rev. B **84**, 085452 (2011).
[S4] E. A. Laird, F. Kuemmeth, G. A. Steele, K. Grove-Rasmussen, J. Nygård, K. Flensberg, and L. P. Kouwenhoven, Rev. Mod. Phys. **87**, 703 (2015).
[S5] D. V. Bulaev, B. Trauzettel, and D. Loss, Phys. Rev. B **77**, 235301 (2008).
[S6] S. Weiss, E. I. Rashba, F. Kuemmeth, H. O. H. Churchill, and K. Flensberg, Phys. Rev. B **82**, 165427 (2010).
[S7] J. S. Lim, R. López, and R. Aguado, Phys. Rev. Lett. **107**, 196801 (2011).
